# Supplementary material for: Recruiting credible participants for field studies in software engineering research
Source: arXiv:2112.14186 source file (2021-12-28)
Supplement: Supplementary file 1 [file Appendix_checklist.tex]

%\clearpage
\section*{Appendix A: Preliminary checklist}

This appendix presents a preliminary checklist that complements the framework discussed in the main article.
% Having presented and discussed a framework for thinking about practitioners as informants in empirical studies, we now present and briefly discuss a preliminary checklist. 
The checklist is intended to be used to assess the extent to which an actual empirical study -- in design, in conduct, or completed -- has considered practitioners as credible participants. The checklist is presented in Table~\ref{table:checklist}. The table does not specify how checklist items might be assessed and, in practice, some items may not be assessable, e.g., assessing the participant's information--processing abilities. In general, we expect that items would likely be graded, e.g., high, medium, low; or yes, no.

\renewcommand{\thetable}{A1}
\clearpage
\begin{table}[htp]
    \small
    \caption{A checklist for assessing the characteristics of practitioners as credible participants}
    \label{table:checklist}
    \centering
    \begin{tabular}{| p{0.4cm}  p{12.5cm} |}
        \toprule
        \textbf{\#} & \textbf{Question}\\
        \midrule
        \multicolumn{2}{|p{13cm}|}{\emph{Ensure the study considers whether a practitioner has Real, Relevant and Recent experience~\cite{falessi2018empirical}}}\\
    %   \midrule
        1 & Does the practitioner have experience of real--world software practice?\\
        % \multicolumn{2}{|l|}{Relevant experience}\\
        % \hline
        2 & Does the practitioner have experience of situations (specifically, of the actor--technology--activity--artefact configuration) that clearly aligns with the theory and proposition/s being studied by the researcher?\\
        % \multicolumn{2}{|l|}{Real experience}\\
        % \hline
        3 & Does the practitioner have recent (timely) experience?\\
        \midrule
        \multicolumn{2}{|l|}{\emph{Ensure the study considers the role of the practitioner}}\\
        % \hline        
        4 & Is the practitioner a \textit{Performer} within the situation, i.e., an actor in the actor--technology--activity--artefact configuration?\\
        5 & Is the practitioner a non--acting \textit{Observer} somewhere within the situation?\\
        6 & Is the practitioner a non--acting, non--observing \textit{Advisor}, offering experiences drawn from other situations?\\
        \midrule
        \multicolumn{2}{|l|}{\emph{Ensure the study considers the information--processing abilities of the practitioner}}\\
        7 & How willing is the practitioner to openly share information?\\
        8 & What quantity of (real, relevant and timely) experience can the practitioner offer to the research?\\
        9 & How observationally sensitive is the practitioner?\\
        10 & How reflective is the practitioner?\\
        11 & How selective is the practitioner of situations and information?\\
        \midrule
        \multicolumn{2}{|l|}{\emph{Ensure the study considers demographics}}\\
        12 & What are the (relevant to the research) demographics of the practitioner?\\
        \midrule
        \multicolumn{2}{|l|}{\emph{Ensure the study considers the number of situations}}\\
        13 & Does the research require practitioners to provide information on a specified situation or number of situations?\\
        \midrule
        \multicolumn{2}{|p{13cm}|}{\emph{Ensure the study considers the appropriate information to request from the practitioner}}\\
        14 & Does the research seek factual information about specific situations?\\
        15 & Does the research seek beliefs drawn from one situation, or from an an aggregated collection of situations?\\
        \midrule
        \multicolumn{2}{|l|}{\emph{Ensure the study considers context}}\\
        % 15 & How close in proximity are the situations of interest?\\
        % 16 & How close in proximity are the informants?\\
        % 17 & What demographic information is considered?\\
        16 & How does the study describe the relevant context?\\
        17 & How `empirically close' is the situation, or the situations, to the theory and propositions of interest to the researcher?\\
        % \\
        \bottomrule
    \end{tabular}
\end{table}
