# Supplementary material for: Recruiting credible participants for field studies in software engineering research
Source: arXiv:2112.14186 source file (2021-12-28)
Supplement: Supplementary file 2 [file Y_additional_material.tex]

\clearpage
\section*{Additional material}

\subsection{Participants as research instruments}
%\label{subsection:participants-as-research-instruments}
Our interest is in information that participants can provide about events external to the participant, e.g., about the behaviour of software phenomena that they observe. We can \textit{model} a participant as a kind of research instrument, or in D'Andrade's \cite{dandrade1974memory} term, as a `behaviourscope'. We can then think of the participant in terms of: their reliability (how consistently they observe the world) and their validity (how accurately they observe the world); in terms of bias; and in terms of information accuracy.

\subsubsection{Validity and reliability}

Homburg et al. \cite{homburg2012drives} used data from 127 studies across six major marketing and management journals to investigate hypotheses concerning key--informant's reliability and validity in survey studies. Unfortunately, Homburg et al. do not define what they mean by \textit{key informant}. Phillips \cite{phillips1981assessing}, cited by Homburg et al. \cite{homburg2012drives} explain that informants are chosen because they have special qualifications such as particular status, specialized knowledge, or even accessibility to the researcher. We discuss key informants later in this section.

Homburg et al. \cite{homburg2012drives} draw on social cognition theory to identify two concepts central to their research: (1) availability of relevant information and (2) difficulty of retrieval. The availability of relevant information and the difficulty of retrieval of information introduce random error. But they can also introduce systematic error. Where an informant lacks pertinent information or struggles to retrieve such information, these informants may provide a random best guess (thus threatening reliability) or may use some heuristic to guide their response (thus threatening validity).

Relating this to the model in Figure \ref{figure:generalised-karlstrom-and-runeson-figure}:

\begin{enumerate}
    \item For case studies, such as the Karlstr{\"o}m and Runeson \cite{karlstrom2006integrating} reference example, we can have more confidence (in relative terms) that the participants will have relevant information as the participants are part of the cases being studied. Note that there may still be systematic error, e.g., from cultural beliefs present within the respective cases being studied.
    
    \item In interview studies (e.g., \cite{curtis1988field}), we can have more confidence (in relative terms) that the participants will have relevant information as the participants have some relationship with the cases of interest. There may still be systematic error, though the content of that error may be different.

    \item It surveys, it is uncertain as to whether the participants have access to relevant information.
    
\end{enumerate}

For reliability, Homburg et al. \cite{homburg2012drives} propose five sets of factors affecting reliability: (1) construct characteristics, (2) informant characteristics, (3) organizational characteristics, and (4) industry characteristics. Because we also investigate formal considerations, we consider method characteristics as a fifth set. For validity, Homburg et al. \cite{homburg2012drives} focus on their construct characteristics.  A summary of their results are presented in Table \ref{table:homburg-hypotheses}.

\begin{table}[!ht]
    \small
    \caption{Constructs affecting reliability and validity (from  \cite{homburg2012drives})}
    \label{table:homburg-hypotheses}
    \centering
    \begin{tabular}{| p{0.5cm} | p{6.6cm} | }
        \hline
        \textbf{\#} & \textbf{Hypothesis}\\
        \hline
        \hline
        \multicolumn{2}{| l |}{Impact of constructs characteristics on \textbf{reliability}}\\
        H1 & The reliability of key informant responses is greater for constructs pertaining to the present (vs. the past).\\
        H2 & The reliability of key informant responses is greater for objective constructs (vs. more subjective constructs)\\
        H3 & The reliability of key informant responses is greater for constructs pertaining to more salient events (vs. more routine events).\\
        
        \multicolumn{2}{| l |}{Impact of informant characteristics on \textbf{reliability}}\\
        H6 & The reliability of key informant responses is greater for informants in higher hierarchical positions (vs. lower hierarchical positions).\\
        
        \multicolumn{2}{| l |}{Impact of method characteristics on \textbf{reliability}}\\
        H14 & Key informant reliability estimates will be greater if triangulation is conducted using archival data (vs. survey data).\\
        
        \multicolumn{2}{| l |}{Impact of construct characteristics on \textbf{validity}}\\
        H16 & The validity of key informant responses is greater for constructs pertaining to the present (vs. the past).\\
        H17 & The validity of key informant responses is greater for objective constructs (vs. more subjective constructs)\\
        H18 & The validity of key informant responses is greater for constructs pertaining to more salient events (vs. more routine events).\\
  
        \hline
    \end{tabular}
\end{table}


\subsubsection{Bias}

Mohanani et al. \cite{mohanani2018cognitive} report a systematic mapping study of cognitive biases in software engineering. Chattopadhyay et al. \cite{chattopadhyay2020tale} report a two--part field of the presence of cognitive biases in software development, drawing on the work of Mohanani et al. \cite{mohanani2018cognitive}. Mohanani et al. cite Flesichmann et al.'s \cite{fleischmann2014cognitive} work.


\begin{table}[!ht]
    \small
    \caption{Cognitive bias (\cite{mohanani2018cognitive}, see also \cite{fleischmann2014cognitive}}
    %\label{table:cognitive-biase}
    \centering
    \begin{tabular}{| p{0.5cm} | p{1cm} | p{5.4cm} | }
        \hline
        \textbf{\#} & \textbf{Bias} & \textbf{Description}\\
        \hline
        \hline
        1  & Stability & Biases that lead individuals to persevere with established or familiar options despite the presence of superior information, arguments or conditions.\\
        2  & Action--oriented & Biases that lead individuals to premature decisions without considering relevant information or alternative courses of action.\\
        3 & Pattern--recognition & Biases that lead individuals to attend more to information that is familiar.\\
        4 & Perception & Biases that prejudice the processing of new information.\\
        5 & Memory & Biases that affect recall of information or experience.\\
        \hline
    \end{tabular}
\end{table}

\subsubsection{Information accuracy}

Bernard et al. \cite{bernard1984problem} are concerned with the validity and accuracy of the ``naive senses'' of informants.  They review previous work in three areas: recall of child care behavior; recall of health seeking behavior; and recall of communication and social interactions. They identify a number of concerns with the use of informants. As an illustrative example, we quote their summary of a study by Kornfield: ``Informants showed much higher agreement about what waiters were wearing than about what waitresses were wearing, despite the fact that none of the restaurants in question had waiters. Informants provided greater detail about the kind of music that was playing in restaurants that, in fact, did not have music than they provided for restaurants that did have music.'' (\cite{bernard1984problem}, p. 509)

We summarise Bernard et al.'s \cite{bernard1984problem} more relevant concerns here:
\begin{enumerate}
    \item Informants \textit{are} inaccurate; memory \textit{does} decay exponentially with time.
    \item There appears to be systematic distortion in how informants recall just about everything.
    \item Recall may be effected by the subject of the study, by whether informants are aided in their recall in some way during the interview, by whether they keep diaries, by conditions of the interview, or by a variety of cultural factors.
    \item If informants agree with one another in information that they independently provide, then there must be a basis for this. The two likely explanations are norms and actual experience.
    \begin{enumerate}
        \item When informants don't recall an actual experience, they are more likely to rely on a cultural norm for their answer.
        \item Informants who have an actual experience are more likely to resist badgering (are less likely to `back down'). A consequence is that answers that show more resistance to badgering is more likely to be accurate.
    \end{enumerate}
    \item Knowing which informants are likely to be least accurate is surely important; but knowing whether \textit{any} informant is sufficiently accurate to rely upon his or her responses is more important still.
    \item Interviewing many inaccurate informants will not solve the accuracy/validity problem
\end{enumerate}

Bernard et al.'s \cite{bernard1984problem}'s observation about cultural norms is demonstrably present in software engineering. For example, Rainer et al. \cite{rainer2003persuading} found that practitioners prefer local opinion over other sources of knowledge. Devanbu et al. \cite{devanbu2016belief} conducted a large survey of Microsoft employees (n=564) finding that developers beliefs are based primarily on their personal experience and then, second, on their peers' opinions. (By contrast, research papers were ranked fifth out of six.)

\subsection{Key informants}

Marshall \cite{marshall1996key} defines a key informant as an expert source of information. He identifies five characteristics of ideal key informants as well as strengths and weaknesses. These are all summarised in Table \ref{table:key-informants}.

In software engineering research, an example of the use of key informants would be an expert panel, e.g., \cite{li2003ranking}.

\begin{table}[!ht]
    \small
    \caption{Characteristics of ideal key informants, and strengths and weaknesses (from \cite{marshall1996key}}
    %\label{table:key-informants}
    \centering
    \begin{tabular}{| l | p{7cm} | }
        \hline
        \textbf{\#} & \textbf{Description}\\
        \hline
        \hline
        \multicolumn{2}{|l|}{Characteristics}\\
        C1 & \textbf{Role in community}. Their formal role should expose them to the kind of information being sought by the researcher\\
        C2 & \textbf{Knowledge}. In addition to having access to the information desired, the informant should have absorbed the information meaningfully.\\
        C3 & \textbf{Willingness}. The informant should be willing to communicate their knowledge to the interviewer and to cooperate as fully as possible.\\
        C4 & \textbf{Communicability}. They should be able to communicate their knowledge in a manner that is intelligible to the interviewer.\\
        C5 & \textbf{Impartiality}. Key informants should be objective and unbiased. Any relevant biases should be known to the interviewer\\
        \hline
        \multicolumn{2}{|l|}{Advantages}\\
        A1 & Quality of data that can be obtained in a relatively short period of time. To obtain the same amount of information and insight from in-depth interviews with other members of a community can be prohibitively time-consuming and expensive\\
        \hline
        \multicolumn{2}{|l|}{Disadvantages}\\
        D1 & Unlikely to represent, or even understand, the majority view of those individuals in their community.\\
        D2 & The identification of key informants may be in error because some societies may attract people who wish to improve their status but do not have the necessary skills of a true key informant\\
        D3 & Informants are different to informers, who are more likely to be biased and to have their own agenda.\\
        D4 & Key informants might only divulge information that is politically acceptable and social rules could discourage the researcher from publishing potentially sensitive data which may be ascribed to a particular informant.\\
        \hline
    \end{tabular}
\end{table}

% \subsection{Relevant knowledge}
% In this subsection we draw on Devanbu et al., Rainer et al., Hoda's paper on recruiting participants to talk about relevant knowledge.

\subsection{Summary}

We need more credible participants for our studies, i.e., informants who are more reliable and who can provide more valid information. Such information is the foundation of empirical work that relies on practitioners, e.g., interviews, focus groups, surveys. `Input' information from practitioners that is invalid, or information for which its validity is highly uncertain, fundamentally undermines the validity of our subsequent research findings, regardless of the reliability of the research process. (Essentially, we have Garbage In, Garbage Out.) Rephrasing Bernard et al. \cite{bernard1984problem}, many studies all reporting invalid findings will not solve the problem. 

Treating the recruitment of participants as a matter of better sampling, so as to `produce' a more representative sample, is potentially mis--framing the problem. This is because participants are often not the target population. In our studies, we are often interested in what participants can tell us \textit{about} our target population, e.g., what an informant tells us about requirements engineering, or software testing, or software projects, or defects.

As a step toward addressing these concerns, we propose a framework and checklist to help researchers think about the recruitment of credible participants.
